# Supplementary material for: SABAF: Removing Strong Attribute Bias from Neural Networks with Adversarial Filtering
Source: arXiv:2311.07141 source file (2023-11-16)
Supplement: Supplementary file 1 [file Adult_supp.tex]

\begin{figure}[htbp]
    \begin{minipage}{0.48\textwidth}
        \centering
        \includegraphics[width=\linewidth]{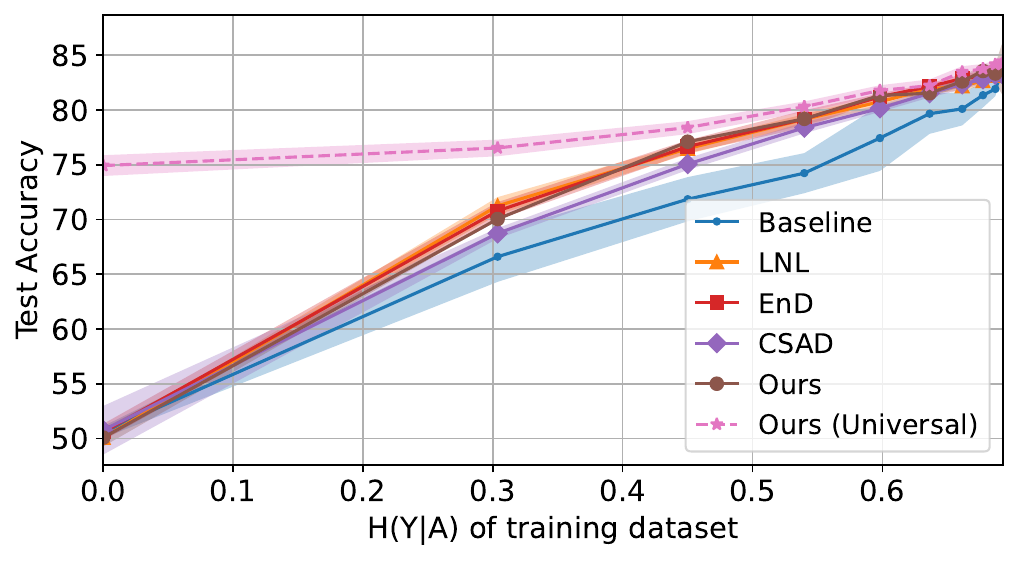}
        \caption{Accuracy of \emph{Unbiased} testing set under different bias strengths in Adult.}
        \label{fig:EB_Adult_unbiased_supp}
    \end{minipage}%
    \hspace{0.3cm}
    \begin{minipage}{0.48\textwidth}
        \centering
        \includegraphics[width=\linewidth]{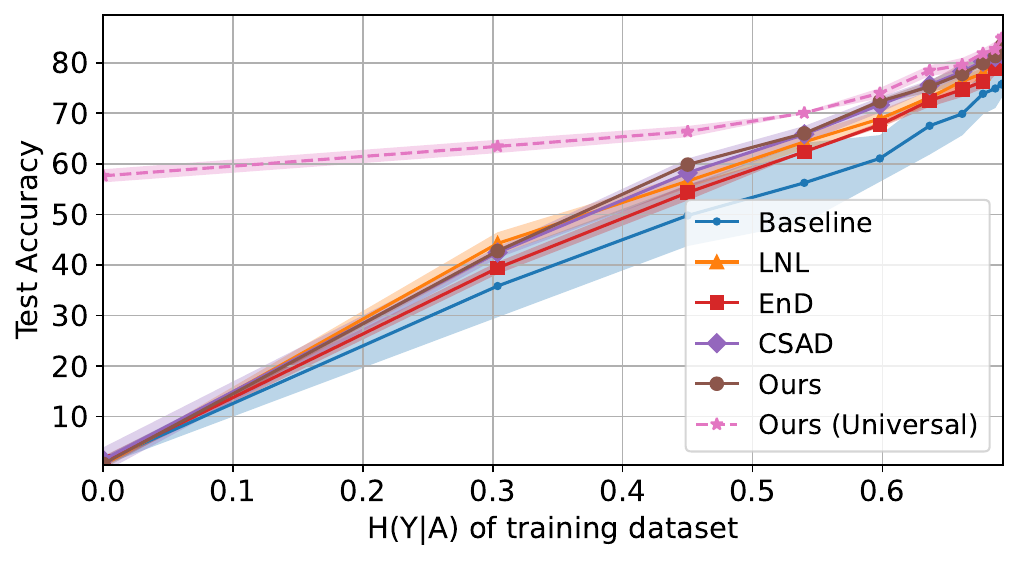}
        \caption{Accuracy of \emph{Bias-conflicting} testing set under different bias strengths in Adult.}
        \label{fig:EB_Adult_biasconflicting_supp}
    \end{minipage}%
\end{figure}

\begin{table}[htbp]
        \caption{Accuracy under extreme bias in Adult. \textbf{Bold} for the best results.}
        \label{tab:Adult_mostEx_supp}
        \centering
        % \resizebox{0.7\textwidth}{!}{%
\begin{tabular}{lcc}
\toprule
                         & Unbiased            & Bias-conflicting    \\
                         \midrule
Baseline                 & 50.59{\scriptsize $\pm$ 0.54}          & 1.19{\scriptsize $\pm$ 0.83}           \\
% DR                       & 66.38{\scriptsize $\pm$ 0.22}          & 38.17{\scriptsize $\pm$ 1.04}          \\
LNL~\cite{learn_not_to_learn_Colored_MNIST}                       & 50.10{\scriptsize $\pm$ 0.18}          & 0.43{\scriptsize $\pm$ 0.46}          \\
EnD~\cite{End}                      & 50.59{\scriptsize $\pm$ 0.75}          & 1.18{\scriptsize $\pm$ 0.96}           \\
CSAD~\cite{CSAD}                     & 50.76{\scriptsize $\pm$ 2.22}          & 1.43{\scriptsize $\pm$ 2.46}           \\
Ours                     & 50.09{\scriptsize $\pm$ 0.81}          & 0.64{\scriptsize $\pm$ 1.01}           \\
\midrule
Ours (Universal) & \textbf{74.93{\scriptsize $\pm$ 0.95}} & \textbf{57.63{\scriptsize $\pm$ 1.30}} \\
\bottomrule
\end{tabular}
        % }
    \end{table}
